# Supplementary material for: Reducing Polarization on Abortion, Guns and Immigration: An Experimental Study
Source: arXiv:2206.13652 source file (2023-02-14)
Supplement: Supplementary file 1 [file APPENDIX_surveys.pdf]

# Survey 1: Eliciting Views on Human Rights and Etiquette Rules

---

**Start of Block: Default Question Block**

Instructions
Thank you for participating in this study titled “Views and attitudes in the United States”, led by researchers at Cornell University and the University of Chicago.

**What the study is about:** The purpose of this study is to understand how people form opinions about various topics of general interest. You will be asked how much you agree or disagree with a list of statements. We will then ask you a few questions about yourself and your experience with the study. You must complete the survey to be compensated for your time. The data collected from this study will be used to write academic research papers.

**What we are asking you to do:** You will be asked to answer a number of survey questions. It should take you less than 10 minutes to complete the study.

**Risks and discomfort:** We anticipate that your participation in this survey presents no greater risk than everyday use of the Internet. You will be compensated as explained by the email you received from your panel provider.

**Benefits:** There are no direct benefits of participating to the study except for the compensation you have been promised to receive as a participant of your panel provider. The main benefit will be to contribute to the scientific knowledge and understanding of how people form opinions in the United States.

**Data Protection / Confidentiality:** Please note that you have been recruited because you are a member of your survey panel. Your survey panel provider has its own privacy and security policies that you can find on its website. Anonymized and de-identified data from this study will be made available to the research community at large to advance science. We will remove or code any personal information that could identify you before files are shared with other researchers to ensure that, by current scientific standards and known methods, no one will be able to identify you from the information we share. Despite these measures, we cannot fully guarantee anonymity of your personal data.

**Taking part is voluntary:** Your involvement is voluntary. You can choose to not participate, discontinue at any time, or skip any questions/procedures that may make you feel uncomfortable.

**Questions?** If you have questions, you can contact the researchers leading this study at mb2693@cornell.edu. If you have any questions or concerns regarding your rights as a subject in this study, you may contact the Institutional Review Board (IRB) for Human Participants at 607-255-5138 or access their website at http://www.irb.cornell.edu. You may also report your concerns or complaints anonymously through Ethicspoint online at www.hotline.cornell.edu or by calling toll free at 1-866-293-3077. Ethicspoint is an independent organization that serves as a liaison between the University and the person bringing the complaint so that anonymity can be ensured.

---

PCF Please indicate your consent to proceed with the study:

- ◯ I have read the information above and consent to participate
- ◯ I do not consent to participate

*Skip To: End of Block If Please indicate your consent to proceed with the study: = I do not consent to participate*

**End of Block: Default Question Block**

---

**Start of Block: Block 4**

state In which state do you currently reside?

▼ Alabama ... I do not reside in the United States

*Skip To: End of Block If 50 States, D.C. and Puerto Rico = I do not reside in the United States*

---

*

zipcode What is your ZIP code?

________________________________________________________________

---

age Please, indicate your age group

- Below 18
- 18-23
- 24-29
- 30-35
- 35-39
- 40-44
- 45-54
- 55-59
- 60 or more
- Prefer not to answer

*Skip To: End of Block If Please, indicate your age group = Below 18*

gender What is your sex?

- Male
- Female
- Other
- Prefer not to answer

race What is your race?

- ☐ White
- ☐ Black or African American
- ☐ American Indian or Alaska Native
- ☐ Asian
- ☐ Native Hawaiian or Pacific Islander
- ☐ Hispanic
- ☐ Prefer not to answer
- ☐ Other ________________________________________________

---

income What was the income of your household in 2020 (before taxes)?

- ○ Less than $16,000
- ○ $16,000 to $31,000
- ○ $31,000 to $50,000
- ○ $50,000 to $70,000
- ○ Over $70,000

---

party Generally speaking, do you usually think of yourself as a Republican, a Democrat, an Independent, or something else?

- ◯ Strong Republican
- ◯ Republican or leaning Republican
- ◯ Independent
- ◯ Democrat or leaning Democrat
- ◯ Strong Democrat
- ◯ Other (please specify) ________________________________________________
- ◯ Prefer not to answer

---

*Display This Question:*

*If Generally speaking, do you usually think of yourself as a Republican, a Democrat, an Independent,... = Democrat or leaning Democrat*

*Or Generally speaking, do you usually think of yourself as a Republican, a Democrat, an Independent,... = Independent*

*Or Generally speaking, do you usually think of yourself as a Republican, a Democrat, an Independent,... = Strong Democrat*

vote_D Which of the following was your preferred Presidential candidate at the last Democratic primaries elections?

- ◯ Joe Biden
- ◯ Bernie Sanders
- ◯ Elizabeth Warren
- ◯ Michael Bloomberg
- ◯ Amy Klobuchar
- ◯ Pete Buttigieg
- ◯ Andrew Yang
- ◯ Prefer not to answer
- ◯ Other (please specify) ________________________________________________

---

*Display This Question:*

*If Generally speaking, do you usually think of yourself as a Republican, a Democrat, an Independent,... = Strong Republican*

*Or Generally speaking, do you usually think of yourself as a Republican, a Democrat, an Independent,... = Republican or leaning Republican*

*Or Generally speaking, do you usually think of yourself as a Republican, a Democrat, an Independent,... = Independent*

vote_R Which of the following was your preferred Presidential candidate at the 2016 primaries elections?

- ○ Donald J. Trump
- ○ Ted Cruz
- ○ Marco Rubio
- ○ Jeb Bush
- ○ Rand Paul
- ○ Ben Carson
- ○ John Kasich
- ○ Prefer not to answer
- ○ Other (please specify) ________________________________________________

**End of Block: Block 4**

---

**Start of Block: Please indicate how much you agree or disagree with the following statements:**

freeeq All human beings are born free and equal in dignity and rights. They are endowed with reason and conscience and should act towards one another in a spirit of brotherhood.

0 (strongly disagree) to 10 (strongly agree)

| | 0 | 1 | 2 | 3 | 4 | 5 | 6 | 7 | 8 | 9 | 10 |
|---|---|---|---|---|---|---|---|---|---|---|---|
| 1 | | | | | | | | | | | |

lifeliberty Everyone has the right to life, liberty and security of person.

0 (strongly disagree) to 10 (strongly agree)

0 1 2 3 4 5 6 7 8 9 10

| | |
|---|---|
| 1 | |

slavery No one shall be held in slavery or servitude; slavery and slave trade shall be prohibited in all their forms.

| | 0 (strongly disagree) to 10 (strongly agree) |
|---|---|
| | 0 1 2 3 4 5 6 7 8 9 10 |
| | |

torture No one shall be subjected to torture or to cruel, inhuman or degrading treatment or punishment.

| | 0 (strongly disagree) to 10 (strongly agree) |
|---|---|
| | 0 1 2 3 4 5 6 7 8 9 10 |
| | |

Page Break

marriage Men and women of full age, without any limitation due to race, nationality or religion, have the right to marry and to found a family. They are entitled to equal rights as to marriage, during marriage and at its dissolution.

0 (strongly disagree) to 10 (strongly agree)

| | 0 | 1 | 2 | 3 | 4 | 5 | 6 | 7 | 8 | 9 | 10 |
|---|---|---|---|---|---|---|---|---|---|---|---|
| | | | | | | | | | | | |

family

The family is the natural and fundamental group unit of society and is entitled to protection by society and the State.

0 (strongly disagree) to 10 (strongly agree)

| | 0 | 1 | 2 | 3 | 4 | 5 | 6 | 7 | 8 | 9 | 10 |
|---|---|---|---|---|---|---|---|---|---|---|---|
| 4 | | | | | | | | | | | |

property

No one shall be arbitrarily deprived of his property.

0 (strongly disagree) to 10 (strongly agree)

| | 0 | 1 | 2 | 3 | 4 | 5 | 6 | 7 | 8 | 9 | 10 |
|---|---|---|---|---|---|---|---|---|---|---|---|
| | | | | | | | | | | | |

religion Everyone has the right to freedom of thought, conscience and religion; this right includes freedom to change his religion or belief, and freedom, either alone or in community with others and in public or private, to manifest his religion or belief in teaching, practice, worship and observance.

| | 0 (strongly disagree) to 10 (strongly agree) |
|---|---|
| | 0 1 2 3 4 5 6 7 8 9 10 |

opinion Everyone has the right to freedom of opinion and expression; this right includes freedom to hold opinions without interference and to seek, receive and impart information and ideas through any media and regardless of frontiers.

| | 0 (strongly disagree) to 10 (strongly agree) |
|---|---|
| | 0 1 2 3 4 5 6 7 8 9 10 |

Page Break

assembly
Everyone has the right to freedom of peaceful assembly and association.

0 (strongly disagree) to 10 (strongly agree)

0 1 2 3 4 5 6 7 8 9 10

voting
The will of the people shall be the basis of the authority of government; this will shall be expressed in periodic and genuine elections which shall be by universal and equal suffrage and shall be held by secret vote or by equivalent free voting procedures.

0 (strongly disagree) to 10 (strongly agree)

0 1 2 3 4 5 6 7 8 9 10

Page Break

work
 Everyone has the right to work, to free choice of employment, to just and favorable conditions of work and to protection against unemployment.

| | 0 (strongly disagree) to 10 (strongly agree) |
| --- | --- |
| | 0 1 2 3 4 5 6 7 8 9 10 |
| | |

---

leisure
 Everyone has the right to rest and leisure, including reasonable limitation of working hours and periodic holidays with pay.

| | 0 (strongly disagree) to 10 (strongly agree) |
| --- | --- |
| | 0 1 2 3 4 5 6 7 8 9 10 |
| | |

---

culture
 Everyone has the right to freely to participate in the cultural life of the community, to enjoy the arts and to share in scientific advancement and its benefits.

| | 0 (strongly disagree) to 10 (strongly agree) |
| --- | --- |
| | 0 1 2 3 4 5 6 7 8 9 10 |
| | |

**End of Block: Please indicate how much you agree or disagree with the following statements:**

---

**Start of Block: Block 3**

etiquettes We now ask you to indicate how much you agree with the following rules of etiquette. In life, it is important to...

| | 0 (strongly disagree) to 10 (strongly agree)<br>0 1 2 3 4 5 6 7 8 9 10 |
|---|---|
| Wait your turn in a waiting line | |
| Hold the door for a person following you | |
| Avoid using your cellphone while you're enjoying a friend's company | |
| Say "please" when you ask for something. | |
| Say "thank you" to acknowledge service, kindness, or the receipt of something. | |
| Arrive on time. Not being late for classes, intimate gatherings, or appointments. | |
| Refrain from chewing or speaking with your mouth open. | |
| Refrain from talking loudly in quiet settings (or on your cell phone in movies, plays, or other quiet or focused communal settings) | |
| Look people in the eye when talking to them | |
| Stand at least a foot away when you are talking to someone you don't know | |

**End of Block: Block 3**

---

**Start of Block: Finally, we would like to ask you about your experience with this survey:**

difficulty Overall, did you find the statements in this survey easy or difficult to understand?

- ○ Very easy
- ○ Easy
- ○ Somewhat easy
- ○ Somewhat difficult
- ○ Difficult
- ○ Very difficult

**End of Block: Finally, we would like to ask you about your experience with this survey:**

# Survey 2: Collecting Recordings

Start of Block: Default Question Block

PIS Thank you for participating in this study titled “Views and attitudes in the United States”, led by researchers at Cornell University and the University of Chicago.

**What the study is about**: The purpose of this study is to understand how people form opinions about various topics of general interest. The data collected from this study will be used to write academic research papers.

**What we are asking you to do**: It should take you less than 10 minutes to complete the study. You will be asked to answer a number of survey questions. We will then ask you to record a short audio of yourself explaining why you support or oppose a specific public policy. Then you will be asked a few questions about yourself and your experience with the study. You must complete the survey to be compensated for your time.

**Risks and discomfort**: We anticipate that your participation in this survey presents no greater risk than everyday use of the Internet. You will be compensated as explained by the email you received from your survey panel provider.

**Benefits**: There are no direct benefits of participating to the study except for the compensation you have been promised to receive as a participant of your panel provider. The main benefit will be to contribute to the scientific knowledge and understanding of how people form opinions in the United States.

**Data Protection / Confidentiality**: Please note that you have been recruited because you are a member of the survey panel provider. Your provider has its own privacy and security policies that you can find on its website. Anonymized and de-identified data from this study will be made available to the research community at large to advance science. We will remove or code any personal information that could identify you before files are shared with other researchers to ensure that, by current scientific standards and known methods, no one will be able to identify you from the information we share. Despite these measures, we cannot fully guarantee anonymity of your personal data.

**Taking part is voluntary**: Your involvement is voluntary. You can choose to not participate, discontinue at any time, or skip any questions/procedures that may make you feel uncomfortable.

**Questions?** If you have questions, you can contact the researchers leading this study at mb2693@cornell.edu. If you have any questions or concerns regarding your rights as a subject in this study, you may contact the Institutional Review Board (IRB) for Human Participants at 607-255-5138 or access their website at http://www.irb.cornell.edu. You may also report your concerns or complaints anonymously through Ethicspoint online at www.hotline.cornell.edu or by calling toll free at 1-866-293-3077. Ethicspoint is an independent organization that serves as a liaison between the University and the person bringing the complaint so that anonymity can be ensured.

---

PCF Please indicate your consent to proceed with the study:

○ I have read the information above and consent to participate

○ I do not consent to participate

*Skip To: End of Block If Please indicate your consent to proceed with the study: = I do not consent to participate*

---

Page Break

state In which state do you currently reside?

▼ Alabama ... I do not reside in the United States

*Skip To: End of Block If 50 States, D.C. and Puerto Rico = I do not reside in the United States*

device To show you the most suitable instructions to complete this survey, please tell us on which device you are currently using to take part in this survey:

- ○ iPhone or iPad
- ○ Android smartphone or Tablet
- ○ Laptop or PC

age Please indicate your age group

- ○ Below 18
- ○ 18-25
- ○ 26-34
- ○ 35-45
- ○ 46-54
- ○ 55-64
- ○ 65-70
- ○ 71-80
- ○ 81 or more
- ○ Prefer not to answer

gender What is your sex?

- ○ Male
- ○ Female
- ○ Other
- ○ Prefer not to answer

race What is your race?

- ☐ White
- ☐ Black or African American
- ☐ American Indian or Alaska Native
- ☐ Asian
- ☐ Native Hawaiian or Pacific Islander
- ☐ Mixed race
- ☐ Hispanic American
- ☐ Prefer not to answer
- ☐ Other ________________________________________________

Page Break

instructions1 In the next four questions we would like to ask you your opinion about four policies. You can move the slider left or right depending on how close your opinion is to the wording provided above the values 0 and 10.

---

abortion In most cases, abortion should be:

| | Illegal | | | | | | Legal | | | | |
|---|---|---|---|---|---|---|---|---|---|---|---|
| | 0 | 1 | 2 | 3 | 4 | 5 | 6 | 7 | 8 | 9 | 10 |
| 1 | | | | | | | | | | | |

---

*Display This Question:*

*If If What is your ZIP code? Text Response Is Equal to 00000*

guns Current gun laws in the United States are

| | Too strict | | | | | | Too lenient | | | | |
|---|---|---|---|---|---|---|---|---|---|---|---|
| | 0 | 1 | 2 | 3 | 4 | 5 | 6 | 7 | 8 | 9 | 10 |
| | | | | | | | | | | | |

---

trade Free trade agreements between the US and other countries have generally been

| | A bad thing | | | | | | A good thing | | | | |
|---|---|---|---|---|---|---|---|---|---|---|---|
| | 0 | 1 | 2 | 3 | 4 | 5 | 6 | 7 | 8 | 9 | 10 |
| | | | | | | | | | | | |

---

*Display This Question:*

*If If What is your ZIP code? Text Response Is Equal to  0000*

immig Legal immigrants in the United States today

| | Burden the country by taking jobs, health care and housing | | | | | | | | | | Strengthen the country through hard work and talent |
|---|---|---|---|---|---|---|---|---|---|---|---|
| | 0 | 1 | 2 | 3 | 4 | 5 | 6 | 7 | 8 | 9 | 10 |
| | | | | | | | | | | | |

End of Block: Default Question Block

Start of Block: Block 2

topic In a previous question you said that you feel strongly about ${e://Field/topic_fill}.

For the next question, we'd like you to share an audio file of yourself expressing, in about 60 seconds or less, your views about the topic.

How would you explain your point of view about this topic to someone else?

*Display This Question:*

*If To show you the most suitable instructions to complete this survey, please tell us on which devic... = iPhone or iPad*

instructions_iphone

*Display This Question:*

*If To show you the most suitable instructions to complete this survey, please tell us on which devic... = Android smartphone or Tablet*

instructions_android

*Display This Question:*

*If To show you the most suitable instructions to complete this survey, please tell us on which devic... = Laptop or PC*

instructions_pc

upload Please upload here below an audio file (of about 60 seconds or less) sharing your views on the topic we just showed you. After uploading the file, make sure you hit the "SUBMIT" button and then the arrow at the bottom of the page to continue.

Page Break

End of Block: Block 2

Start of Block: Block 3

zipcode What is your ZIP code?

________________________________________________________________

educ What is your (highest) level of education?

- Elementary school
- Middle school
- High school
- Higher education (non University)
- Higher education (University)
- Prefer not to answer

income What was the income of your household in 2020 (before taxes)?

- Less than $16,000
- $16,000 to $31,000
- $31,000 to $50,000
- $50,000 to $70,000
- Over $70,000

party Generally speaking, do you usually think of yourself as a Republican, a Democrat, an Independent, or something else?

- ◯ Strong Republican
- ◯ Republican or leaning Republican
- ◯ Independent
- ◯ Democrat or leaning Democrat
- ◯ Strong Democrat
- ◯ Other (please specify) ________________________________________________
- ◯ Prefer not to answer

**End of Block: Block 3**

---

# Survey 3: Main Study

---

Start of Block: PIS_PCF

Q1 Thank you for participating in this study titled “Views and attitudes in the United States”, led by researchers at Cornell University and the University of Chicago.

**What the study is about**: The purpose of this study is to understand how people form opinions about various topics of general interest. The data collected from this study will be used to write academic research papers.

**What we are asking you to do**: It should take you less than 10 minutes to complete the study. You will be asked to answer a number of survey questions. We will then show you some audio files that you can choose to listen to or not. Then you will be asked a few questions about yourself and your experience with the study. You must complete the survey to be compensated for your time.

**Risks and discomfort**: We anticipate that your participation in this survey presents no greater risk than everyday use of the Internet. You will be compensated as explained by the email you received from your survey panel provider.

**Benefits**: There are no direct benefits of participating to the study except for the compensation you have been promised to receive as a participant of your panel provider. The main benefit will be to contribute to the scientific knowledge and understanding of how people form opinions in the United States.

**Data Protection / Confidentiality**: Please note that you have been recruited because you are a member of the survey panel provider. Your provider has its own privacy and security policies that you can find on its website. Anonymized and de-identified data from this study will be made available to the research community at large to advance science. We will remove or code any personal information that could identify you before files are shared with other researchers to ensure that, by current scientific standards and known methods, no one will be able to identify you from the information we share. Despite these measures, we cannot fully guarantee anonymity of your personal data.

**Taking part is voluntary**: Your involvement is voluntary. You can choose to not participate,

discontinue at any time, or skip any questions/procedures that may make you feel uncomfortable.

**Questions?** If you have questions, you can contact the researchers leading this study at mb2693@cornell.edu. If you have any questions or concerns regarding your rights as a subject in this study, you may contact the Institutional Review Board (IRB) for Human Participants at 607-255-5138 or access their website at http://www.irb.cornell.edu. You may also report your concerns or complaints anonymously through Ethicspoint online at www.hotline.cornell.edu or by calling toll free at 1-866-293-3077. Ethicspoint is an independent organization that serves as a liaison between the University and the person bringing the complaint so that anonymity can be ensured.

---

Q2 Please indicate your consent to proceed with the study:

○ I have read the information above and consent to participate

○ I do not consent to participate

*Skip To: End of Block If Please indicate your consent to proceed with the study: = I do not consent to participate*

---

Page Break

End of Block: PIS_PCF

Start of Block: UN and etiquettes

instruction Please indicate how much you agree or disagree (0 is strongly disagree and 10 is strongly agree) with the following statements:

slavery No one shall be held in slavery or servitude; slavery and slave trade shall be prohibited in all their forms.

| | Strongly disagree | | | | | | | | | Strongly agree | |
|---|---|---|---|---|---|---|---|---|---|---|---|
| | 0 | 1 | 2 | 3 | 4 | 5 | 6 | 7 | 8 | 9 | 10 |
| | | | | | | | | | | | |

property
No one shall be arbitrarily deprived of his property.

| | Strongly disagree | | | | | | | | | Strongly agree | |
|---|---|---|---|---|---|---|---|---|---|---|---|
| | 0 | 1 | 2 | 3 | 4 | 5 | 6 | 7 | 8 | 9 | 10 |
| | | | | | | | | | | | |

assembly
Everyone has the right to freedom of peaceful assembly and association.

| | Strongly disagree | | | | | | | | | Strongly agree | |
|---|---|---|---|---|---|---|---|---|---|---|---|
| | 0 | 1 | 2 | 3 | 4 | 5 | 6 | 7 | 8 | 9 | 10 |
| | | | | | | | | | | | |

lifeliberty Everyone has the right to life, liberty and security of person.

| | Strongly disagree | | | | | Strongly agree | | | | | |
|---|---|---|---|---|---|---|---|---|---|---|---|
| | 0 | 1 | 2 | 3 | 4 | 5 | 6 | 7 | 8 | 9 | 10 |
| 1 | | | | | | | | | | | |

culture
Everyone has the right to freely to participate in the cultural life of the community, to enjoy the arts and to share in scientific advancement and its benefits.

| | Strongly disagree | | | | | Strongly agree | | | | | |
|---|---|---|---|---|---|---|---|---|---|---|---|
| | 0 | 1 | 2 | 3 | 4 | 5 | 6 | 7 | 8 | 9 | 10 |
| | | | | | | | | | | | |

Page Break

etiq_waitline We now ask you to indicate how much you agree with the following rules of etiquette, on a scale from 0 (strongly disagree) to 10 (strongly agree).

In life, it is important to wait your turn in a waiting line.

Strongly disagree Strongly agree

0 1 2 3 4 5 6 7 8 9 10

---

etiq_sayplease In life, it is important to say “please” when you ask for something.

Strongly disagree Strongly agree

0 1 2 3 4 5 6 7 8 9 10

---

etiq_saythanks In life, it is important to say “thank you” to acknowledge service, kindness, or the receipt of something.

Strongly disagree Strongly agree

0 1 2 3 4 5 6 7 8 9 10

---

etiq_ontime In life, it is important to arrive on time. Not being late for classes, intimate gatherings, or appointments.

Strongly disagree Strongly agree

0 1 2 3 4 5 6 7 8 9 10

etiq_talkloud In life, it is important to refrain from talking loudly in quiet settings (or on your cell phone in movies, plays, or other quiet or focused communal settings)/

| | Strongly disagree | Strongly agree |
| --- | --- | --- |
| | 0 1 2 3 4 5 | 6 7 8 9 10 |
| | | |

End of Block: UN and etiquettes

Start of Block: policies

intro_policies We would now like to ask you your opinion about three policies. You can move the slider left or right depending on how close your opinion is to the wording provided above the values 0 and 10.

abortion In most cases, abortion should be:

| | Illegal | Legal |
| --- | --- | --- |
| | 0 1 2 3 4 5 | 6 7 8 9 10 |
| 1 | | |

guns Current gun laws in the United States are

| | Too strict | Too lenient |
| --- | --- | --- |
| | 0 1 2 3 4 5 | 6 7 8 9 10 |

immigration Legal immigrants in the United States today

| | Burden the country by taking jobs, health care and housing | | | | | | | | | | Strengthen the country through hard work and talent |
|---|---|---|---|---|---|---|---|---|---|---|---|
| | 0 | 1 | 2 | 3 | 4 | 5 | 6 | 7 | 8 | 9 | 10 |

End of Block: policies

Start of Block: audio_instructions

audio_instructions

**<u>Please read these instructions carefully.</u>**

In the next pages of the survey, you will have the opportunity to listen to three recordings from people who have views that differ from yours on the policy issues we asked you about (immigration, gun laws and abortion). Each recording lasts less than 1 minute.

You can choose to listen to none, all, or only some of these files.

Make sure you have your audio on or you are wearing headphones
should you choose to listen to the files.

audio_instr_timer Timing
First Click
Last Click
Page Submit
Click Count

End of Block: audio_instructions

Start of Block: instructions_control

instructions_control Click the 'next' button to begin.

C_instructionstimer Timing
First Click
Last Click
Page Submit
Click Count

End of Block: instructions_control

Start of Block: instructions_T1_etiq

instructions_T1_etiq In a previous question we asked how much you agreed with a set of behavioral etiquettes, such as saying 'thank you', 'please', and arriving on time.

We asked these exact same questions to the people who recorded the audio files you will be shown in the next pages and each of them had a rate of agreement above 9 out of 10.

That is, they also strongly agree that in life it is important to:

- Wait your turn in a waiting line
- Say “please” when you ask for something.
- Say “thank you” to acknowledge service, kindness, or the receipt of something.
- Arrive on time. Not being late for classes, intimate gatherings, or appointments.
- Refrain from talking loudly in quiet settings (or on your cell phone in movies, plays, or other quiet or focused communal settings)

Click the 'next' button to begin.

T1_instructionstimer Timing
First Click
Last Click
Page Submit
Click Count

End of Block: instructions_T1_etiq

Start of Block: instructions_T2_UN

instructions_T2_UN Earlier in this survey we asked how much you agreed with a set of human principles, such as banning slavery, protecting private property, and freedom of association.

We asked these exact same questions to the people who recorded the audio files you will be shown in the next pages and each of them had an average rate of agreement with these principles between 9 and 10.

That is, they strongly agreed that:

- No one shall be held in slavery or servitude; slavery and slave trade shall be prohibited in all their forms.
- No one shall be arbitrarily deprived of his property.
- Everyone has the right to freedom of peaceful assembly and association.
- Everyone has the right to life, liberty and security of person.
- Everyone has the right to freely to participate in the cultural life of the community, to enjoy the arts and to share in scientific advancement and its benefits.
  Click the 'next' button to begin.

---

instructions_T2timer Timing
First Click
Last Click
Page Submit
Click Count

End of Block: instructions_T2_UN

Start of Block: audio 6

audio6
This recording is from an American resident who believes that in most cases abortion should be <u>legal</u>.

---

timer_audio6 Timing
First Click
Last Click
Page Submit
Click Count

End of Block: audio 6

---

Start of Block: audio 16

audio16
This recording is from an American resident who believes that in most cases abortion should be legal.

---

timer_audio16 Timing
First Click
Last Click
Page Submit
Click Count

End of Block: audio 16

---

Start of Block: audio 17

audio17
This recording is from an American resident who believes that in most cases abortion should be legal.

---

timer_audio17 Timing
First Click
Last Click
Page Submit
Click Count

End of Block: audio 17

---

Start of Block: audio 20

audio20
This recording is from an American resident who believes that in most cases abortion should be legal.

---

timer_audio20 Timing
First Click
Last Click
Page Submit
Click Count

End of Block: audio 20

Start of Block: audio 30

audio30
This recording is from an American resident who believes that in most cases abortion should be legal.

---

timer_audio30 Timing
First Click
Last Click
Page Submit
Click Count

End of Block: audio 30

Start of Block: audio 43

audio43
This recording is from an American resident who believes that in most cases abortion should be legal.

---

timer_audio43 Timing
First Click
Last Click
Page Submit
Click Count

End of Block: audio 43

---

Start of Block: audio 46

audio46
This recording is from an American resident who believes that in most cases abortion should be legal.

timer_audio46 Timing
First Click
Last Click
Page Submit
Click Count

End of Block: audio 46

---

Start of Block: audio 9

audio9
This recording is from an American resident who believes that in most cases abortion should be illegal.

timer_audio9 Timing
First Click
Last Click
Page Submit
Click Count

End of Block: audio 9

---

Start of Block: audio 10

audio10
This recording is from an American resident who believes that in most cases abortion should be illegal.

timer_audio10 Timing
First Click
Last Click
Page Submit
Click Count

**End of Block: audio 10**

**Start of Block: audio 15**

audio15
This recording is from an American resident who believes that in most cases abortion should be illegal.

timer_audio15 Timing
First Click
Last Click
Page Submit
Click Count

**End of Block: audio 15**

**Start of Block: audio 18**

audio18
This recording is from an American resident who believes that in most cases abortion should be illegal.

timer_audio18 Timing
First Click
Last Click
Page Submit
Click Count

End of Block: audio 18

---

Start of Block: audio 19

audio19
This recording is from an American resident who believes that in most cases abortion should be illegal.

---

timer_audio19 Timing
First Click
Last Click
Page Submit
Click Count

End of Block: audio 19

---

Start of Block: audio 21

audio21
This recording is from an American resident who believes that in most cases abortion should be illegal.

---

timer_audio21 Timing
First Click
Last Click
Page Submit
Click Count

End of Block: audio 21

---

Start of Block: audio 34

audio34
This recording is from an American resident who believes that in most cases abortion should be illegal.

timer_audio34 Timing
First Click
Last Click
Page Submit
Click Count

End of Block: audio 34

Start of Block: audio 36

audio36
This recording is from an American resident who believes that in most cases abortion should be illegal.

timer_audio36 Timing
First Click
Last Click
Page Submit
Click Count

End of Block: audio 36

Start of Block: audio 37

audio37
This recording is from an American resident who believes that in most cases abortion should be illegal.

timer_audio37 Timing
First Click
Last Click
Page Submit
Click Count

End of Block: audio 37

---

Start of Block: audio 38

audio38
This recording is from an American resident who believes that in most cases abortion should be illegal.

---

timer_audio38 Timing
First Click
Last Click
Page Submit
Click Count

End of Block: audio 38

---

Start of Block: audio 5

audio5
This recording is from an American resident who believes that legal immigrants in the United States today strengthen the country through hard work and talent.

---

timer_audio5 Timing
First Click
Last Click
Page Submit
Click Count

End of Block: audio 5

---

Start of Block: audio 7

audio7
This recording is from an American resident who believes that legal immigrants in the United States today strengthen the country through hard work and talent.

---

timer_audio7 Timing
First Click
Last Click
Page Submit
Click Count

**End of Block: audio 7**

---

**Start of Block: audio 8**

audio8
This recording is from an American resident who believes that legal immigrants in the United States today strengthen the country through hard work and talent.

---

timer_audio8 Timing
First Click
Last Click
Page Submit
Click Count

**End of Block: audio 8**

---

**Start of Block: audio 11**

audio11
This recording is from an American resident who believes that legal immigrants in the United States today strengthen the country through hard work and talent.

---

timer_audio11 Timing
First Click
Last Click
Page Submit
Click Count

End of Block: audio 11

---

Start of Block: audio 24

audio24
This recording is from an American resident who believes that legal immigrants in the United States today strengthen the country through hard work and talent.

timer_audio24 Timing
First Click
Last Click
Page Submit
Click Count

End of Block: audio 24

---

Start of Block: audio 27

audio27
This recording is from an American who believes that legal immigrants in the United States today strengthen the country through hard work and talent.

timer_audio27 Timing
First Click
Last Click
Page Submit
Click Count

End of Block: audio 27

---

Start of Block: audio 28

audio28
This recording is from an American resident who believes that legal immigrants in the United States today strengthen the country through hard work and talent.

timer_audio28 Timing
First Click
Last Click
Page Submit
Click Count

End of Block: audio 28

Start of Block: audio 29

audio29
This recording is from an American who believes that legal immigrants in the United States today strengthen the country through hard work and talent.

timer_audio29 Timing
First Click
Last Click
Page Submit
Click Count

End of Block: audio 29

Start of Block: audio 32

audio32
This recording is from an American resident who believes that legal immigrants in the United States today strengthen the country through hard work and talent.

timer_audio32 Timing
First Click
Last Click
Page Submit
Click Count

End of Block: audio 32

---

Start of Block: audio 3

audio3
This recording is from an American resident who believes that legal immigrants in the United States today burden the country by taking jobs, health care and housing.

---

timer_audio3 Timing
First Click
Last Click
Page Submit
Click Count

End of Block: audio 3

---

Start of Block: audio 13

audio13
This recording is from an American resident who believes that legal immigrants in the United States today burden the country by taking jobs, health care and housing.

---

timer_audio13 Timing
First Click
Last Click
Page Submit
Click Count

End of Block: audio 13

---

Start of Block: audio 23

audio23
 This recording is from an American resident who believes that legal immigrants in the United States today burden the country by taking jobs, health care and housing.

---

timer_audio23 Timing
First Click
Last Click
Page Submit
Click Count

**End of Block: audio 23**

---

**Start of Block: audio 40**

audio40
 This recording is from an American resident who believes that legal immigrants in the United States today burden the country by taking jobs, health care and housing.

---

timer_audio40 Timing
First Click
Last Click
Page Submit
Click Count

**End of Block: audio 40**

---

**Start of Block: audio 2**

audio2
This recording is from an American resident who believes that current gun laws in the United States are too lenient.

---

timer_audio2 Timing
First Click
Last Click
Page Submit
Click Count

End of Block: audio 2

---

Start of Block: audio 14

audio14
This recording is from an American resident who believes that current gun laws in the United States are too lenient.

---

timer_audio14 Timing
First Click
Last Click
Page Submit
Click Count

End of Block: audio 14

---

Start of Block: audio 22

audio22
This recording is from an American resident who believes that current gun laws in the United States are too lenient.

---

timer_audio22 Timing
First Click
Last Click
Page Submit
Click Count

End of Block: audio 22

---

Start of Block: audio 25

audio25
This recording is from an American resident who believes that current gun laws in the United States are too lenient.

---

timer_audio25 Timing
First Click
Last Click
Page Submit
Click Count

End of Block: audio 25

---

Start of Block: audio 31

audio31
This recording is from an American resident who believes that current gun laws in the United States are too lenient.

---

timer_audio31 Timing
First Click
Last Click
Page Submit
Click Count

End of Block: audio 31

---

Start of Block: audio 33

audio33
This recording is from an American resident who believes that current gun laws in the United States are too lenient.

---

timer_audio33 Timing
First Click
Last Click
Page Submit
Click Count

**End of Block: audio 33**

---

**Start of Block: audio 44**

audio44
This recording is from an American resident who believes that current gun laws in the United States are too lenient.

---

timer_audio44 Timing
First Click
Last Click
Page Submit
Click Count

**End of Block: audio 44**

---

**Start of Block: audio 47**

audio47
This recording is from an American resident who believes that current gun laws in the United States are too lenient.

---

timer_audio47 Timing
First Click
Last Click
Page Submit
Click Count

**End of Block: audio 47**

---

**Start of Block: audio 1**

audio1
 This recording is from an American resident who believes that current gun laws in the United States are too strict.

---

timer_audio1 Timing
First Click
Last Click
Page Submit
Click Count

**End of Block: audio 1**

---

**Start of Block: audio 4**

audio4
 This recording is from an American resident who believes that current gun laws in the United States are too strict.

---

timer_audio4 Timing
First Click
Last Click
Page Submit
Click Count

**End of Block: audio 4**

---

**Start of Block: audio 26**

audio26
This recording is from an American resident who believes that current gun laws in the United States are too strict.

---

timer_audio26 Timing
First Click
Last Click
Page Submit
Click Count

End of Block: audio 26

---

Start of Block: audio 35

audio35
This recording is from an American resident who believes that current gun laws in the United States are too strict.

---

timer_audio35 Timing
First Click
Last Click
Page Submit
Click Count

End of Block: audio 35

---

Start of Block: audio 39

audio39
This recording is from an American resident who believes that current gun laws in the United States are too strict.

---

timer_audio39 Timing
First Click
Last Click
Page Submit
Click Count

End of Block: audio 39

---

Start of Block: audio 41

audio41
This recording is from an American resident who believes that current gun laws in the United States are too strict.

timer_audio41 Timing
First Click
Last Click
Page Submit
Click Count

End of Block: audio 41

Start of Block: audio 42

audio42
This recording is from an American resident who believes that current gun laws in the United States are too strict.

timer_audio42 Timing
First Click
Last Click
Page Submit
Click Count

End of Block: audio 42

Start of Block: audio 45

audio45
This recording is from an American resident who believes that current gun laws in the United States are too strict.

timer_audio45 Timing
First Click
Last Click
Page Submit
Click Count

End of Block: audio 45

Start of Block: audio 12

audio12
This recording is from an American resident who believes that current gun laws in the United States are too strict.

timer_audio12 Timing
First Click
Last Click
Page Submit
Click Count

End of Block: audio 12

Start of Block: policies_post

which_listened_to Which audio files have you listened to?

| | I listened to all of it | I listened to some of it | I did not listen to it |
|---|---|---|---|
| Immigration | ○ | ○ | ○ |
| Gun laws | ○ | ○ | ○ |
| Abortion | ○ | ○ | ○ |

End of Block: policies_post

Start of Block: changed_views_immigration

changed_views_imm Has listening to the recording on immigration changed your views?

- ◯ Yes
- ◯ No
- ◯ I did not listen to it

End of Block: changed_views_immigration

---

Start of Block: changed_views_guns

changed_views_guns Has listening to the recording on gun laws changed your views?

- ◯ Yes
- ◯ No
- ◯ I did not listen to it

End of Block: changed_views_guns

---

Start of Block: changed_views_abortion

changed_views_abort Has listening to the recording on abortion changed your views?

- ◯ Yes
- ◯ No
- ◯ I did not listen to it

End of Block: changed_views_abortion

---

Start of Block: post_abortion_no

post_abortion_no Please indicate why your views on abortion have not changed:

○ I already knew and considered the arguments presented

○ I didn't find the arguments convincing

○ Other ________________________________________________

End of Block: post_abortion_no

---

Start of Block: post_guns_no

post_guns_no Please indicate why your views on gun laws have not changed:

○ I already knew and considered the arguments presented

○ I didn't find the arguments convincing

○ Other ________________________________________________

End of Block: post_guns_no

---

Start of Block: post_immigration_no

post_immigration_no Please indicate why your views on immigration have not changed:

○ I already knew and considered the arguments presented

○ I didn't find the arguments convincing

○ Other ________________________________________________

End of Block: post_immigration_no

---

Start of Block: post_guns_yes

post_guns Please indicate how you feel now.

Current gun laws in the United States are:

| | Too strict | | | | | | | | | | Too lenient |
|---|---|---|---|---|---|---|---|---|---|---|---|
| | 0 | 1 | 2 | 3 | 4 | 5 | 6 | 7 | 8 | 9 | 10 |

End of Block: post_guns_yes

Start of Block: post_abortion_yes

post_abortion Please indicate how you feel now.

In most cases, abortion should be:

| | Illegal | | | | | | | | Legal | | |
|---|---|---|---|---|---|---|---|---|---|---|---|
| | 0 | 1 | 2 | 3 | 4 | 5 | 6 | 7 | 8 | 9 | 10 |
| 1 | | | | | | | | | | | |

End of Block: post_abortion_yes

Start of Block: post_immigration_yes

post_immigration Please indicate how you feel now.

Legal immigrants in the United States today

| | Burden the country by taking jobs, health care and housing | | | | | | | | | Strengthen the country through hard work and talent | |
|---|---|---|---|---|---|---|---|---|---|---|---|
| | 0 | 1 | 2 | 3 | 4 | 5 | 6 | 7 | 8 | 9 | 10 |
| | | | | | | | | | | | |

End of Block: post_immigration_yes

Start of Block: Affective polarization

Thermometer We’d like you to rate how you feel towards the Democratic and Republican parties on a scale of 0 to 100, which we call a "feeling thermometer."

On this feeling thermometer scale, ratings between 0 and 49 degrees mean that you feel unfavorable and cold (with 0 being the most unfavorable/coldest). Ratings between 51 and 100 degrees mean that you feel favorable and warm (with 100 being the most favorable/warmest). A rating of 50 means you have no feelings one way or the other.

How would you rate your feeling toward the Democratic and Republican parties?

| | 0 10 20 30 40 50 60 70 80 90 100 |
|---|---|
| Democratic party | |
| Republican party | |

End of Block: Affective polarization

Start of Block: demographics block

demo_intro Thank you for taking part in this survey until now. We would now like to ask you few last questions about yourself. This and the next page are the last ones of the survey.

state In which state do you currently reside?

▼ Alabama ... I do not reside in the United States

race What is your race? Select all that apply.

- ☐ White
- ☐ Black or African American
- ☐ American Indian or Alaska Native
- ☐ Asian
- ☐ Native Hawaiian or Pacific Islander
- ☐ Hispanic American
- ☐ Prefer not to answer
- ☐ Other ________________________________________________

age Please indicate your age group

- Below 18
- 18-25
- 26-34
- 35-45
- 46-54
- 55-64
- 65-70
- 71-80
- 81 or more
- Prefer not to answer

*Skip To: End of Block If Please indicate your age group = Below 18*

gender What is your sex?

- Male
- Female
- Other
- Prefer not to answer

educ What is your (highest) level of education?

- ○ Elementary school
- ○ Middle school
- ○ High school
- ○ Higher education (non University)
- ○ Higher education (University)
- ○ Prefer not to answer

---

zipcode What is your ZIP code?

________________________________________________________________

---

income What was the income of your household in 2020 (before taxes)?

- ○ Less than $16,000
- ○ $16,000 to $31,000
- ○ $31,000 to $50,000
- ○ $50,000 to $70,000
- ○ Over $70,000

---

party Generally speaking, do you usually think of yourself as a Republican, a Democrat, an Independent, or something else?

- Strong Republican
- Republican or leaning towards Republican
- Centrist
- Democrat or leaning towards Democrat
- Strong Democrat
- Independent
- Other (please specify): ________________________________________________

---

vote Are you allowed to vote in Presidential elections in the U.S.?

- Yes
- No

**End of Block: demographics block**
